# Supplementary material for: Geometric optimization using nonlinear rotation-invariant coordinates
Source: arXiv:1908.11728 ancillary file (2020-04-28)
Supplement: Supplementary file 1 [file Derivatives.pdf]

# Supplementary Material: Geometric optimization using nonlinear rotation-invariant coordinates

## Derivatives of the transition rotations and the nonlinear energy

Josua Sassen, Behrend Heeren, Klaus Hildebrandt, Martin Rumpf

### 1 Transition rotations

In this part of the supplementary material, we provide the derivatives of the induced transition rotations in quaternion form alluded to in the main text. Remember, there we derived the representation

$$\hat{q}(\theta, a, b, c) = \cos \frac{\theta}{2} \sqrt{\frac{1+Q(a, b, c)}{2}} + \sin \frac{\theta}{2} \sqrt{\frac{1+Q(a, b, c)}{2}} \mathbf{i} - \sin \frac{\theta}{2} \sqrt{\frac{1-Q(a, b, c)}{2}} \mathbf{j} + \cos \frac{\theta}{2} \sqrt{\frac{1-Q(a, b, c)}{2}} \mathbf{k}.$$

where  $a, b$ , and  $c$  are the edge lengths,  $\theta$  is the dihedral angle, and  $Q(a, b, c) = \frac{a^2+b^2-c^2}{2ab}$  is the cosine of the interior angle opposite to  $c$ . We computed the derivatives of these rotations using MATHEMATICA and present the results below. Contrary to before, we represent the derivatives as vectors  $(a, b, c, d) \in \mathbb{R}^4$  to obtain a more readable representation. The corresponding MATHEMATICA notebook is also included in the supplementary material.

Before we get started, let us introduce some important abbreviations. First, we denote by  $A_f$  the triangle computed using Heron's formula, *i.e.*

$$A_f := A(a, b, c) := \frac{1}{4} \sqrt{(a+b+c)(-a+b+c)(a-b+c)(a+b-c)}. \quad (1)$$

Furthermore, we use  $Q$  for the cosine of the interior angle without stating the dependence on  $a, b$ , and  $c$  explicitly, *i.e.*

$$Q := Q(a, b, c) := \frac{a^2 + b^2 - c^2}{2ab}. \quad (2)$$

#### 1.1 Local first derivatives

We compute the following derivatives as

$$\partial_\theta \hat{q}(\theta, a, b, c) = \frac{1}{2} \begin{pmatrix} -\sin\left(\frac{\theta}{2}\right) \sqrt{\frac{1+Q}{2}} \\ \cos\left(\frac{\theta}{2}\right) \sqrt{\frac{1+Q}{2}} \\ -\cos\left(\frac{\theta}{2}\right) \sqrt{\frac{1-Q}{2}} \\ -\sin\left(\frac{\theta}{2}\right) \sqrt{\frac{1-Q}{2}} \end{pmatrix},$$

and

$$\partial_a \hat{q}(\theta, a, b, c) = \frac{S_2}{8aA_f} \begin{pmatrix} \cos\left(\frac{\theta}{2}\right) \sqrt{\frac{1-Q}{2}} \\ \sin\left(\frac{\theta}{2}\right) \sqrt{\frac{1-Q}{2}} \\ \sin\left(\frac{\theta}{2}\right) \sqrt{\frac{1+Q}{2}} \\ -\cos\left(\frac{\theta}{2}\right) \sqrt{\frac{1+Q}{2}} \end{pmatrix},$$

and

$$\partial_b \hat{q}(\theta, a, b, c) = \frac{S_1}{8bA_f} \begin{pmatrix} \cos\left(\frac{\theta}{2}\right) \sqrt{\frac{1-Q}{2}} \\ \sin\left(\frac{\theta}{2}\right) \sqrt{\frac{1-Q}{2}} \\ \sin\left(\frac{\theta}{2}\right) \sqrt{\frac{1+Q}{2}} \\ -\cos\left(\frac{\theta}{2}\right) \sqrt{\frac{1+Q}{2}} \end{pmatrix},$$

and lastly

$$\partial_c \hat{q}(\theta, a, b, c) = \frac{c}{4A_f} \begin{pmatrix} -\cos\left(\frac{\theta}{2}\right) \sqrt{\frac{1-Q}{2}} \\ -\sin\left(\frac{\theta}{2}\right) \sqrt{\frac{1-Q}{2}} \\ -\sin\left(\frac{\theta}{2}\right) \sqrt{\frac{1+Q}{2}} \\ \cos\left(\frac{\theta}{2}\right) \sqrt{\frac{1+Q}{2}} \end{pmatrix}.$$

## 1.2 Local second derivatives

For the second derivatives, we have

$$\partial_\theta \partial_\theta \hat{q}(\theta, a, b, c) = \frac{1}{4} \begin{pmatrix} -\cos\left(\frac{\theta}{2}\right) \sqrt{\frac{1+Q}{2}} \\ -\sin\left(\frac{\theta}{2}\right) \sqrt{\frac{1+Q}{2}} \\ \sin\left(\frac{\theta}{2}\right) \sqrt{\frac{1-Q}{2}} \\ -\cos\left(\frac{\theta}{2}\right) \sqrt{\frac{1-Q}{2}} \end{pmatrix},$$

$$\partial_a \partial_\theta \hat{q}(\theta, a, b, c) = \frac{S_2}{16aA_f} \begin{pmatrix} -\sin\left(\frac{\theta}{2}\right) \sqrt{\frac{1-Q}{2}} \\ \cos\left(\frac{\theta}{2}\right) \sqrt{\frac{1-Q}{2}} \\ \cos\left(\frac{\theta}{2}\right) \sqrt{\frac{1+Q}{2}} \\ \sin\left(\frac{\theta}{2}\right) \sqrt{\frac{1+Q}{2}} \end{pmatrix},$$

$$\partial_b \partial_\theta \hat{q}(\theta, a, b, c) = \frac{S_1}{16bA_f} \begin{pmatrix} -\sin\left(\frac{\theta}{2}\right) \sqrt{\frac{1-Q}{2}} \\ \cos\left(\frac{\theta}{2}\right) \sqrt{\frac{1-Q}{2}} \\ \cos\left(\frac{\theta}{2}\right) \sqrt{\frac{1+Q}{2}} \\ \sin\left(\frac{\theta}{2}\right) \sqrt{\frac{1+Q}{2}} \end{pmatrix},$$

$$\partial_c \partial_\theta \hat{q}(\theta, a, b, c) = \frac{c}{8A_f} \begin{pmatrix} \sin\left(\frac{\theta}{2}\right) \sqrt{\frac{1-Q}{2}} \\ -\cos\left(\frac{\theta}{2}\right) \sqrt{\frac{1-Q}{2}} \\ -\cos\left(\frac{\theta}{2}\right) \sqrt{\frac{1+Q}{2}} \\ -\sin\left(\frac{\theta}{2}\right) \sqrt{\frac{1+Q}{2}} \end{pmatrix},$$

$$\partial_a \partial_a \hat{q}(\theta, a, b, c) = \frac{1}{128a^2A_f^3} \begin{pmatrix} \cos\left(\frac{\theta}{2}\right) \left( S_3 S_2^2 \sqrt{\frac{1-Q}{2}} - 2A_f S_2^2 \sqrt{\frac{1+Q}{2}} + 32A_f^2 (b^2 - c^2) \sqrt{\frac{1-Q}{2}} \right) \\ \sin\left(\frac{\theta}{2}\right) \left( S_3 S_2^2 \sqrt{\frac{1-Q}{2}} - 2A_f S_2^2 \sqrt{\frac{1+Q}{2}} + 32A_f^2 (b^2 - c^2) \sqrt{\frac{1-Q}{2}} \right) \\ \sin\left(\frac{\theta}{2}\right) \left( S_3 S_2^2 \sqrt{\frac{1+Q}{2}} + 2A_f S_2^2 \sqrt{\frac{1-Q}{2}} + 32A_f^2 (b^2 - c^2) \sqrt{\frac{1+Q}{2}} \right) \\ \cos\left(\frac{\theta}{2}\right) \left( -S_3 S_2^2 \sqrt{\frac{1+Q}{2}} - 2A_f S_2^2 \sqrt{\frac{1-Q}{2}} - 32A_f^2 (b^2 - c^2) \sqrt{\frac{1+Q}{2}} \right) \end{pmatrix},$$

$$\begin{aligned}
\partial_b \partial_a \hat{q}(\theta, a, b, c) &= \frac{1}{64abA_f^3} \begin{pmatrix} \cos\left(\frac{\theta}{2}\right) \left( -4a^2b^2c^2 \sqrt{\frac{1-Q}{2}} - A_f S_1 S_2 \sqrt{\frac{1+Q}{2}} \right) \\ \sin\left(\frac{\theta}{2}\right) \left( -4a^2b^2c^2 \sqrt{\frac{1-Q}{2}} - A_f S_1 S_2 \sqrt{\frac{1+Q}{2}} \right) \\ -\sin\left(\frac{\theta}{2}\right) \left( 4a^2b^2c^2 \sqrt{\frac{1+Q}{2}} - A_f S_1 S_2 \sqrt{\frac{1-Q}{2}} \right) \\ \cos\left(\frac{\theta}{2}\right) \left( 4a^2b^2c^2 \sqrt{\frac{1+Q}{2}} - A_f S_1 S_2 \sqrt{\frac{1-Q}{2}} \right) \end{pmatrix}, \\
\partial_c \partial_a \hat{q}(\theta, a, b, c) &= \frac{c}{32aA_f^3} \begin{pmatrix} \cos\left(\frac{\theta}{2}\right) \left( a^2 S_1 \sqrt{\frac{1-Q}{2}} + A_f S_2 \sqrt{\frac{1+Q}{2}} \right) \\ \sin\left(\frac{\theta}{2}\right) \left( a^2 S_1 \sqrt{\frac{1-Q}{2}} + A_f S_2 \sqrt{\frac{1+Q}{2}} \right) \\ -\sin\left(\frac{\theta}{2}\right) \left( -a^2 S_1 \sqrt{\frac{1+Q}{2}} + A_f S_2 \sqrt{\frac{1-Q}{2}} \right) \\ \cos\left(\frac{\theta}{2}\right) \left( -a^2 S_1 \sqrt{\frac{1+Q}{2}} + A_f S_2 \sqrt{\frac{1-Q}{2}} \right) \end{pmatrix}, \\
\partial_b \partial_b \hat{q}(\theta, a, b, c) &= \frac{1}{128b^2 A_f^3} \begin{pmatrix} \cos\left(\frac{\theta}{2}\right) \left( S_3 S_1^2 \sqrt{\frac{1-Q}{2}} - 2A_f S_1^2 \sqrt{\frac{1+Q}{2}} + 32A_f^2 (a^2 - c^2) \sqrt{\frac{1-Q}{2}} \right) \\ \sin\left(\frac{\theta}{2}\right) \left( S_3 S_1^2 \sqrt{\frac{1-Q}{2}} - 2A_f S_1^2 \sqrt{\frac{1+Q}{2}} + 32A_f^2 (a^2 - c^2) \sqrt{\frac{1-Q}{2}} \right) \\ \sin\left(\frac{\theta}{2}\right) \left( S_3 S_1^2 \sqrt{\frac{1+Q}{2}} + 2A_f S_1^2 \sqrt{\frac{1-Q}{2}} + 32A_f^2 (a^2 - c^2) \sqrt{\frac{1+Q}{2}} \right) \\ \cos\left(\frac{\theta}{2}\right) \left( -S_3 S_1^2 \sqrt{\frac{1+Q}{2}} - 2A_f S_1^2 \sqrt{\frac{1-Q}{2}} - 32A_f^2 (a^2 - c^2) \sqrt{\frac{1+Q}{2}} \right) \end{pmatrix}, \\
\partial_c \partial_b \hat{q}(\theta, a, b, c) &= \frac{c}{32bA_f^3} \begin{pmatrix} \cos\left(\frac{\theta}{2}\right) \left( b^2 S_2 \sqrt{\frac{1-Q}{2}} + A_f S_1 \sqrt{\frac{1+Q}{2}} \right) \\ \sin\left(\frac{\theta}{2}\right) \left( b^2 S_2 \sqrt{\frac{1-Q}{2}} + A_f S_1 \sqrt{\frac{1+Q}{2}} \right) \\ -\sin\left(\frac{\theta}{2}\right) \left( -b^2 S_2 \sqrt{\frac{1+Q}{2}} + A_f S_1 \sqrt{\frac{1-Q}{2}} \right) \\ -\cos\left(\frac{\theta}{2}\right) \left( b^2 S_2 \sqrt{\frac{1+Q}{2}} - A_f S_1 \sqrt{\frac{1-Q}{2}} \right) \end{pmatrix}, \text{ and} \\
\partial_c \partial_c \hat{q}(\theta, a, b, c) &= \frac{1}{64A_f^3} \begin{pmatrix} -\cos\left(\frac{\theta}{2}\right) \left( 4c^2 A_f \sqrt{\frac{1+Q}{2}} + S_1 S_2 \sqrt{\frac{1-Q}{2}} \right) \\ -\sin\left(\frac{\theta}{2}\right) \left( 4c^2 A_f \sqrt{\frac{1+Q}{2}} + S_1 S_2 \sqrt{\frac{1-Q}{2}} \right) \\ \sin\left(\frac{\theta}{2}\right) \left( 4c^2 A_f \sqrt{\frac{1-Q}{2}} - S_1 S_2 \sqrt{\frac{1+Q}{2}} \right) \\ -\cos\left(\frac{\theta}{2}\right) \left( 4c^2 A_f \sqrt{\frac{1-Q}{2}} - S_1 S_2 \sqrt{\frac{1+Q}{2}} \right) \end{pmatrix}
\end{aligned}$$

where

$$\begin{aligned}
S_0 &:= (a^2 + b^2 + c^2) \\
S_1 &:= (-a^2 + b^2 + c^2) \\
S_2 &:= (a^2 - b^2 + c^2) \\
S_3 &:= (a^2 + b^2 - c^2).
\end{aligned}$$

## 2 Membrane Energy

The next task is to compute the derivatives of the local contribution of the membrane energy for each triangle

$$\mathcal{W}_{\text{mem}}^{\text{local}}(a, b, c, \tilde{a}, \tilde{b}, \tilde{c}) := A(a, b, c) \cdot W_{\text{mem}}(\hat{\mathcal{G}}(a, b, c, \tilde{a}, \tilde{b}, \tilde{c})), \quad (3)$$

where again  $a, b, c$  are the edge lengths of the triangle in the undeformed configuration and  $\tilde{a}, \tilde{b}, \tilde{c}$  are the deformed edge lengths. Note, that we directly include the triangle area stemming from the integration in the computation of the derivative.

Again, we will denote by  $A_f$  the area of the undeformed triangle and by  $\tilde{A}_f$  the area of the deformed one, i.e.

$$A_f := A(a, b, c), \quad \tilde{A}_f := A(\tilde{a}, \tilde{b}, \tilde{c}). \quad (4)$$

Furthermore, we will use additional auxiliary variables throughout the computations which shorten the formulas and are also helpful for implementations. Their definitions will be provided afterwards.

### 2.1 First derivatives

We compute the first derivatives as

$$\partial_a \mathcal{W}_{\text{mem}}^{\text{local}} = A_f \left[ \left( \frac{\lambda}{4} \frac{\tilde{A}_f^2}{A_f^2} - \left( \frac{\lambda}{4} + \frac{\mu}{2} \right) \right) S_3 + \frac{\mu}{2} \left( \frac{aX_2 + 2a\tilde{b}^2}{X_1} - X_4 \frac{\tilde{a}^2 b^2 - 0.5X_3 X_2 + a^2 \tilde{b}^2}{X_1^2} \right) \right],$$

$$\partial_b \mathcal{W}_{\text{mem}}^{\text{local}} = A_f \left[ \left( \frac{\lambda}{4} \frac{\tilde{A}_f^2}{A_f^2} - \left( \frac{\lambda}{4} + \frac{\mu}{2} \right) \right) S_2 + \frac{\mu}{2} \left( \frac{bX_2 + 2b\tilde{a}^2}{X_1} - X_5 \frac{\tilde{a}^2 b^2 - 0.5X_3 X_2 + a^2 \tilde{b}^2}{X_1^2} \right) \right],$$

$$\partial_c \mathcal{W}_{\text{mem}}^{\text{local}} = A_f \left[ \left( \frac{\lambda}{4} \frac{\tilde{A}_f^2}{A_f^2} - \left( \frac{\lambda}{4} + \frac{\mu}{2} \right) \right) S_1 + \frac{\mu}{2} \left( cX_3 \frac{\tilde{a}^2 b^2 - 0.5X_3 X_2 + a^2 \tilde{b}^2}{X_1^2} - \frac{cX_2}{X_1} \right) \right],$$

$$\partial_{\tilde{a}} \mathcal{W}_{\text{mem}}^{\text{local}} = A_f \left[ \frac{\mu}{2} \left( \frac{2\tilde{a}b^2 + \tilde{a}X_3}{X_1} \right) - \left( \frac{\lambda}{4} \frac{\tilde{A}_f^2}{A_f^2} - \left( \frac{\lambda}{4} + \frac{\mu}{2} \right) \right) \tilde{S}_3 \right],$$

$$\partial_{\tilde{b}} \mathcal{W}_{\text{mem}}^{\text{local}} = A_f \left[ \frac{\mu}{2} \left( \frac{2a^2 \tilde{b} + \tilde{b}X_3}{X_1} \right) - \left( \frac{\lambda}{4} \frac{\tilde{A}_f^2}{A_f^2} - \left( \frac{\lambda}{4} + \frac{\mu}{2} \right) \right) \tilde{S}_2 \right], \text{ and}$$

$$\partial_{\tilde{c}} \mathcal{W}_{\text{mem}}^{\text{local}} = A_f \left[ -\frac{\mu}{2} \frac{\tilde{c}X_3}{X_1} - \left( \frac{\lambda}{4} \frac{\tilde{A}_f^2}{A_f^2} - \left( \frac{\lambda}{4} + \frac{\mu}{2} \right) \right) \tilde{S}_1 \right].$$

### 2.2 Second derivatives

First, we compute for the second derivatives only involving undeformed edge lengths

$$\begin{aligned} \partial_a \partial_a \mathcal{W}_{\text{mem}}^{\text{local}} = A_f & \left[ 2 \left( \frac{\lambda}{4} + \frac{\mu}{2} + \frac{R}{4} \right) (B_1 + B_2 - B_3 - B_5 - B_6 + B_9) \right. \\ & \left. + \left( \frac{\lambda}{4} + \frac{\mu}{2} + T - \frac{R}{4} \right) (B_4 + B_7 + B_{10} + B_{13}) + \frac{2(-\tilde{a}^2 + \tilde{b}^2 + \tilde{c}^2)\mu}{16A_f^2} (1 + aS_3) \right], \end{aligned}$$

$$\begin{aligned}\partial_b \partial_a \mathcal{W}_{\text{mem}}^{\text{local}} = A_f \left[ 2 \left( \frac{\lambda}{4} + \frac{\mu}{2} + \frac{R}{4} \right) (B_6 + B_1) + \left( \frac{\lambda}{4} + \frac{\mu}{2} + T - \frac{R}{4} \right) (B_4 - B_7 - B_{10} + B_{13}) \right. \\ \left. + \frac{a \left( -\tilde{a}^2 + \tilde{b}^2 + \tilde{c}^2 \right) \mu}{16A_f^2} S_2 + \frac{b \left( \tilde{a}^2 - \tilde{b}^2 + \tilde{c}^2 \right) \mu}{16A_f^2} S_3 \right],\end{aligned}$$

$$\begin{aligned}\partial_c \partial_a \mathcal{W}_{\text{mem}}^{\text{local}} = A_f \left[ 2 \left( \frac{\lambda}{4} + \frac{\mu}{2} + \frac{R}{4} \right) (B_5 + B_2) + \left( \frac{\lambda}{4} + \frac{\mu}{2} + T - \frac{R}{4} \right) (B_4 - B_7 + B_{10} - B_{13}) \right. \\ \left. + \frac{a \left( -\tilde{a}^2 + \tilde{b}^2 + \tilde{c}^2 \right) \mu}{16A_f^2} S_1 + \frac{c \left( \tilde{a}^2 + \tilde{b}^2 - \tilde{c}^2 \right) \mu}{16A_f^2} S_3 \right],\end{aligned}$$

$$\begin{aligned}\partial_b \partial_b \mathcal{W} = A_f \left[ 2 \left( \frac{\lambda}{4} + \frac{\mu}{2} + \frac{R}{4} \right) (B_1 - B_2 + B_3 + B_5 - B_6 - B_9) \right. \\ \left. + \left( \frac{\lambda}{4} + \frac{\mu}{2} + T - \frac{R}{4} \right) (B_4 + B_7 + B_{10} + B_{13}) + \frac{2 \left( \tilde{a}^2 - \tilde{b}^2 + \tilde{c}^2 \right) \mu}{16A_f^2} (1 + bS_2) \right],\end{aligned}$$

$$\begin{aligned}\partial_c \partial_b \mathcal{W} = A_f \left[ 2 \left( \frac{\lambda}{4} + \frac{\mu}{2} + \frac{R}{4} \right) (B_9 + B_3) + \left( \frac{\lambda}{4} + \frac{\mu}{2} + T - \frac{R}{4} \right) (B_4 + B_7 - B_{10} - B_{13}) \right. \\ \left. + \frac{a \left( -\tilde{a}^2 + \tilde{b}^2 + \tilde{c}^2 \right) \mu}{16A_f^2} S_1 + \frac{c \left( \tilde{a}^2 + \tilde{b}^2 - \tilde{c}^2 \right) \mu}{16A_f^2} S_3 \right], \text{ and}\end{aligned}$$

$$\begin{aligned}\partial_c \partial_c \mathcal{W} = \left[ 2A_f \left( \frac{\lambda}{4} + \frac{\mu}{2} + \frac{R}{4} \right) (-B_1 + B_2 + B_3 - B_5 + B_6 - B_9) \right. \\ \left. + A_f \left( \frac{\lambda}{4} + \frac{\mu}{2} + T - \frac{R}{4} \right) (B_4 + B_7 + B_{10} + B_{13}) \right. \\ \left. + A_f \frac{2 \left( \tilde{a}^2 + \tilde{b}^2 - \tilde{c}^2 \right) \mu}{16A_f^2} (1 + cS_1) \right].\end{aligned}$$

Second, we compute for the second derivatives only involving deformed edge lengths

$$\begin{aligned}\partial_{\tilde{a}} \partial_{\tilde{a}} \mathcal{W} = A_f \left[ \frac{\lambda}{2} \frac{\tilde{A}_f^2}{A_f^2} (C_1 + C_2 - C_3 - C_5 - C_6 + C_9) \right. \\ \left. + \left( \frac{\lambda}{4} + \frac{\mu}{2} \right) (C_4 + C_7 + C_{10} + C_{13}) + \frac{2 \left( -a^2 + b^2 + c^2 \right) \mu}{16A_f^2} \right],\end{aligned}$$

$$\partial_{\tilde{b}} \partial_{\tilde{a}} \mathcal{W} = A_f \left[ \frac{\lambda}{2} \frac{\tilde{A}_f^2}{A_f^2} (C_1 + C_6) + \left( \frac{\lambda}{4} + \frac{\mu}{2} \right) (C_4 - C_7 - C_{10} + C_{13}) \right],$$

$$\partial_{\tilde{c}} \partial_{\tilde{a}} \mathcal{W} = A_f \left[ \frac{\lambda}{2} \frac{\tilde{A}_f^2}{A_f^2} (C_2 + C_5) + \left( \frac{\lambda}{4} + \frac{\mu}{2} \right) (C_4 - C_7 + C_{10} - C_{13}) \right],$$

$$\begin{aligned}\partial_{\tilde{b}}\partial_{\tilde{b}}\mathcal{W} = A_f \left[ \frac{\lambda}{2} \frac{\tilde{A}_f^2}{A_f^2} (C_1 - C_2 + C_3 + C_5 - C_6 - C_9) \right. \\ \left. + \left( \frac{\lambda}{4} + \frac{\mu}{2} \right) (C_4 + C_7 + C_{10} + C_{13}) + \frac{2(a^2 - b^2 + c^2)\mu}{16A_f^2} \right],\end{aligned}$$

$$\partial_{\tilde{c}}\partial_{\tilde{b}}\mathcal{W} = A_f \left[ \frac{\lambda}{2} \frac{\tilde{A}_f^2}{A_f^2} (C_3 + C_9) + \left( \frac{\lambda}{4} + \frac{\mu}{2} \right) (C_4 + C_7 - C_{10} - C_{13}) \right], \text{ and}$$

$$\begin{aligned}\partial_{\tilde{c}}\partial_{\tilde{c}}\mathcal{W} = A_f \left[ \frac{\lambda}{2} \frac{\tilde{A}_f^2}{A_f^2} (-C_1 + C_2 + C_3 - C_5 + C_6 - C_9) \right. \\ \left. + \left( \frac{\lambda}{4} + \frac{\mu}{2} \right) (C_4 + C_7 + C_{10} + C_{13}) + \frac{2(a^2 + b^2 - c^2)\mu}{16A_f^2} \right].\end{aligned}$$

Last, we compute the mixed second derivatives

$$\begin{aligned}\partial_{\tilde{a}}\partial_a\mathcal{W} = \frac{A_f}{2} \left( \frac{\lambda}{4} \frac{\tilde{A}_f^2}{A_f^2} + \left( \frac{\lambda}{4} + \frac{\mu}{2} \right) \right) ( & - A_1 - A_2 + A_3 - A_4 + A_5 + A_6 - A_7 + A_8 \\ & - A_9 - A_{10} + A_{11} - A_{12} - A_{13} - A_{14} + A_{15} - A_{16} ) \\ & + \frac{\tilde{a}(-a^2 + b^2 + c^2)\mu}{16A_f} S_3 - \frac{a\tilde{a}\mu}{4A_f},\end{aligned}$$

$$\begin{aligned}\partial_{\tilde{b}}\partial_a\mathcal{W} = \frac{A_f}{2} \left( \frac{\lambda}{4} \frac{\tilde{A}_f^2}{A_f^2} + \left( \frac{\lambda}{4} + \frac{\mu}{2} \right) \right) ( & - A_1 - A_2 + A_3 - A_4 - A_5 - A_6 + A_7 - A_8 \\ & + A_9 + A_{10} - A_{11} + A_{12} - A_{13} - A_{14} + A_{15} - A_{16} ) \\ & + \frac{\tilde{b}(a^2 - b^2 + c^2)\mu}{16A_f} S_3 + \frac{a\tilde{b}\mu}{4A_f},\end{aligned}$$

$$\begin{aligned}\partial_{\tilde{c}}\partial_a\mathcal{W} = \frac{A_f}{2} \left( \frac{\lambda}{4} \frac{\tilde{A}_f^2}{A_f^2} + \left( \frac{\lambda}{4} + \frac{\mu}{2} \right) \right) ( & - A_1 - A_2 + A_3 - A_4 - A_5 - A_6 + A_7 - A_8 \\ & - A_9 - A_{10} + A_{11} - A_{12} + A_{13} + A_{14} - A_{15} + A_{16} ) \\ & + \frac{\tilde{c}(a^2 + b^2 - c^2)\mu}{16A_f} S_3 + \frac{a\tilde{c}\mu}{4A_f},\end{aligned}$$

$$\begin{aligned}\partial_{\tilde{a}}\partial_b\mathcal{W} = \frac{A_f}{2} \left( \frac{\lambda}{4} \frac{\tilde{A}_f^2}{A_f^2} + \left( \frac{\lambda}{4} + \frac{\mu}{2} \right) \right) ( & - A_1 + A_2 - A_3 - A_4 + A_5 - A_6 + A_7 + A_8 \\ & - A_9 + A_{10} - A_{11} - A_{12} - A_{13} + A_{14} - A_{15} - A_{16} ) \\ & + \frac{\tilde{a}(-a^2 + b^2 + c^2)\mu}{16A_f} S_2 + \frac{b\tilde{a}\mu}{4A_f},\end{aligned}$$

$$\begin{aligned}\partial_{\tilde{b}}\partial_b\mathcal{W} = \frac{A_f}{2} \left( \frac{\lambda}{4} \frac{\tilde{A}_f^2}{A_f^2} + \left( \frac{\lambda}{4} + \frac{\mu}{2} \right) \right) ( & - A_1 + A_2 - A_3 - A_4 - A_5 + A_6 - A_7 - A_8 \\ & + A_9 - A_{10} + A_{11} + A_{12} - A_{13} + A_{14} - A_{15} - A_{16} ) \\ & + \frac{\tilde{b}(a^2 - b^2 + c^2)\mu}{16A_f} S_2 - \frac{b\tilde{b}\mu}{4A_f},\end{aligned}$$

$$\begin{aligned} \partial_{\tilde{c}}\partial_b\mathcal{W} = & \frac{A_f}{2} \left( \frac{\lambda}{4} \frac{\tilde{A}_f^2}{A_f^2} + \left( \frac{\lambda}{4} + \frac{\mu}{2} \right) \right) ( \quad - A_1 + A_2 - A_3 - A_4 - A_5 + A_6 - A_7 - A_8 \\ & - A_9 + A_{10} - A_{11} - A_{12} + A_{13} - A_{14} + A_{15} + A_{16} \quad ) \\ & + \frac{\tilde{c}(a^2 + b^2 - c^2)\mu}{16A_f} S_2 + \frac{b\tilde{c}\mu}{4A_f}, \end{aligned}$$

$$\begin{aligned} \partial_{\tilde{a}}\partial_c\mathcal{W} = & \frac{A_f}{2} \left( \frac{\lambda}{4} \frac{\tilde{A}_f^2}{A_f^2} + \left( \frac{\lambda}{4} + \frac{\mu}{2} \right) \right) ( \quad A_1 - A_2 - A_3 - A_4 - A_5 + A_6 + A_7 + A_8 \\ & + A_9 - A_{10} - A_{11} - A_{12} + A_{13} - A_{14} - A_{15} - A_{16} \quad ) \\ & + \frac{\tilde{a}(-a^2 + b^2 + c^2)\mu}{16A_f} S_1 + \frac{c\tilde{a}\mu}{4A_f}, \end{aligned}$$

$$\begin{aligned} \partial_{\tilde{b}}\partial_c\mathcal{W} = & \frac{A_f}{2} \left( \frac{\lambda}{4} \frac{\tilde{A}_f^2}{A_f^2} + \left( \frac{\lambda}{4} + \frac{\mu}{2} \right) \right) ( \quad A_1 - A_2 - A_3 - A_4 + A_5 - A_6 - A_7 - A_8 \\ & - A_9 + A_{10} + A_{11} + A_{12} + A_{13} - A_{14} - A_{15} - A_{16} \quad ) \\ & + \frac{\tilde{b}(a^2 - b^2 + c^2)\mu}{16A_f} S_1 + \frac{c\tilde{b}\mu}{4A_f}, \text{ and} \end{aligned}$$

$$\begin{aligned} \partial_{\tilde{c}}\partial_c\mathcal{W} = & \frac{A_f}{2} \left( \frac{\lambda}{4} \frac{\tilde{A}_f^2}{A_f^2} + \left( \frac{\lambda}{4} + \frac{\mu}{2} \right) \right) ( \quad A_1 - A_2 - A_3 - A_4 + A_5 - A_6 - A_7 - A_8 \\ & + A_9 - A_{10} - A_{11} - A_{12} - A_{13} + A_{14} + A_{15} + A_{16} \quad ) \\ & + \frac{\tilde{c}(a^2 + b^2 - c^2)\mu}{16A_f} S_1 + \frac{c\tilde{c}\mu}{4A_f}. \end{aligned}$$

The remaining derivatives follow by symmetry.

### 2.3 Auxiliary variables

$$\begin{aligned} X_1 &:= a^2b^2 - \frac{1}{4}X_3^2 \\ X_2 &:= (-\tilde{a}^2 - \tilde{b}^2 + \tilde{c}^2) \\ X_3 &:= (-a^2 - b^2 + c^2) \\ X_4 &:= (2ab^2 + aX_3) \\ X_5 &:= (2ba^2 + bX_3) \\ X_6 &:= \left( \frac{1}{2}(-a^2 + b^2 + c^2)\tilde{a}^2 + \frac{1}{2}(a^2 + b^2 - c^2)\tilde{c}^2 + \frac{1}{2}\tilde{b}^2(a^2 - b^2 + c^2) \right) \end{aligned}$$

$$\begin{aligned}
S_1 &:= +\frac{1}{(a+b-c)} - \frac{1}{(a-b+c)} - \frac{1}{(-a+b+c)} - \frac{1}{(a+b+c)} \\
S_2 &:= -\frac{1}{(a+b-c)} + \frac{1}{(a-b+c)} - \frac{1}{(-a+b+c)} - \frac{1}{(a+b+c)} \\
S_3 &:= -\frac{1}{(a+b-c)} - \frac{1}{(a-b+c)} + \frac{1}{(-a+b+c)} - \frac{1}{(a+b+c)} \\
\tilde{S}_1 &:= +\frac{1}{(\tilde{a}+\tilde{b}-\tilde{c})} - \frac{1}{(\tilde{a}-\tilde{b}+\tilde{c})} - \frac{1}{(-\tilde{a}+\tilde{b}+\tilde{c})} - \frac{1}{(\tilde{a}+\tilde{b}+\tilde{c})} \\
\tilde{S}_2 &:= -\frac{1}{(\tilde{a}+\tilde{b}-\tilde{c})} + \frac{1}{(\tilde{a}-\tilde{b}+\tilde{c})} - \frac{1}{(-\tilde{a}+\tilde{b}+\tilde{c})} - \frac{1}{(\tilde{a}+\tilde{b}+\tilde{c})} \\
\tilde{S}_3 &:= -\frac{1}{(\tilde{a}+\tilde{b}-\tilde{c})} - \frac{1}{(\tilde{a}-\tilde{b}+\tilde{c})} + \frac{1}{(-\tilde{a}+\tilde{b}+\tilde{c})} - \frac{1}{(\tilde{a}+\tilde{b}+\tilde{c})}
\end{aligned}$$

$$T := \frac{\lambda}{4} \frac{\tilde{A}_f^2}{A_f^2} - \left( \frac{\lambda}{4} + \frac{\mu}{2} \right) + \frac{2(X_6)\mu}{16A_f^2} \qquad R := T - \frac{\mu}{2} - \left( \frac{\lambda}{4} + \frac{\mu}{2} \right) \log \left( \frac{\tilde{A}_f^2}{A_f^2} \right)$$

$$\begin{aligned}
A_1 &:= \frac{1}{(a+b-c)(\tilde{a}+\tilde{b}+\tilde{c})} & B_1 &:= \frac{1}{(a+b-c)(a+b+c)} & C_1 &:= \frac{1}{(\tilde{a}+\tilde{b}-\tilde{c})(\tilde{a}+\tilde{b}+\tilde{c})} \\
A_2 &:= \frac{1}{(a-b+c)(\tilde{a}+\tilde{b}+\tilde{c})} & B_2 &:= \frac{1}{(a-b+c)(a+b+c)} & C_2 &:= \frac{1}{(\tilde{a}-\tilde{b}+\tilde{c})(\tilde{a}+\tilde{b}+\tilde{c})} \\
A_3 &:= \frac{1}{(-a+b+c)(\tilde{a}+\tilde{b}+\tilde{c})} & B_3 &:= \frac{1}{(-a+b+c)(a+b+c)} & C_3 &:= \frac{1}{(-\tilde{a}+\tilde{b}+\tilde{c})(\tilde{a}+\tilde{b}+\tilde{c})} \\
A_4 &:= \frac{1}{(a+b+c)(\tilde{a}+\tilde{b}+\tilde{c})} & B_4 &:= \frac{1}{(a+b+c)^2} & C_4 &:= \frac{1}{(\tilde{a}+\tilde{b}+\tilde{c})^2} \\
A_5 &:= \frac{1}{(a+b-c)(-\tilde{a}+\tilde{b}+\tilde{c})} & B_5 &:= \frac{1}{(a+b-c)(-a+b+c)} & C_5 &:= \frac{1}{(\tilde{a}+\tilde{b}-\tilde{c})(-\tilde{a}+\tilde{b}+\tilde{c})} \\
A_6 &:= \frac{1}{(a-b+c)(-\tilde{a}+\tilde{b}+\tilde{c})} & B_6 &:= \frac{1}{(a-b+c)(-a+b+c)} & C_6 &:= \frac{1}{(\tilde{a}-\tilde{b}+\tilde{c})(-\tilde{a}+\tilde{b}+\tilde{c})} \\
A_7 &:= \frac{1}{(-a+b+c)(-\tilde{a}+\tilde{b}+\tilde{c})} & B_7 &:= \frac{1}{(-a+b+c)^2} & C_7 &:= \frac{1}{(-\tilde{a}+\tilde{b}+\tilde{c})^2} \\
A_8 &:= \frac{1}{(a+b+c)(-\tilde{a}+\tilde{b}+\tilde{c})} & & & & \\
A_9 &:= \frac{1}{(a+b-c)(\tilde{a}-\tilde{b}+\tilde{c})} & B_9 &:= \frac{1}{(a+b-c)(a-b+c)} & C_9 &:= \frac{1}{(\tilde{a}+\tilde{b}-\tilde{c})(\tilde{a}-\tilde{b}+\tilde{c})} \\
A_{10} &:= \frac{1}{(a-b+c)(\tilde{a}-\tilde{b}+\tilde{c})} & B_{10} &:= \frac{1}{(a-b+c)^2} & C_{10} &:= \frac{1}{(\tilde{a}-\tilde{b}+\tilde{c})^2} \\
A_{11} &:= \frac{1}{(-a+b+c)(\tilde{a}-\tilde{b}+\tilde{c})} & & & & \\
A_{12} &:= \frac{1}{(a+b+c)(\tilde{a}-\tilde{b}+\tilde{c})} & & & & \\
A_{13} &:= \frac{1}{(a+b-c)(\tilde{a}+\tilde{b}-\tilde{c})} & B_{13} &:= \frac{1}{(a+b-c)^2} & C_{13} &:= \frac{1}{(\tilde{a}+\tilde{b}-\tilde{c})^2} \\
A_{14} &:= \frac{1}{(a-b+c)(\tilde{a}+\tilde{b}-\tilde{c})} & & & & \\
A_{15} &:= \frac{1}{(-a+b+c)(\tilde{a}+\tilde{b}-\tilde{c})} & & & & \\
A_{16} &:= \frac{1}{(a+b+c)(\tilde{a}+\tilde{b}-\tilde{c})} & & & &
\end{aligned}$$

### 3 Bending Energy

Finally, we also need the derivatives of the local contribution of the bending energy for each edge  $e \in \mathcal{E}$ . To this end, we denote by  $\theta$  the dihedral angle at  $e$  in the undeformed configuration and by  $\tilde{\theta}$  in the deformed configuration. Furthermore, we denote by  $l_e$  the length of  $e$  in the undeformed configuration, by  $l_1, l_2$  the lengths of the remaining two edges of the triangle left of  $e$ , and by  $r_1, r_2$  the lengths of the remaining edges of the triangle right of  $e$ . Note, that the designation which triangle is left and which is right is arbitrary and does not influence the calculations as long as it is made consistently. The choice which edge of the adjacent triangles are the first or the second in the above indices also does not matter.

From these edge lengths, we can compute the area of the undeformed left triangle

$$A_l := A(l_e, l_1, l_2) \quad (5)$$

and of the undeformed right triangle

$$A_r := A(l_e, r_1, r_2) \quad (6)$$

using Heron's formula. These two can be combined to compute the edge-associated area

$$d_e := d_e(l_e, l_1, l_2, r_1, r_2) := \frac{1}{3}(A_l + A_r). \quad (7)$$

Using this we can write the local contribution for the bending energy as

$$\mathcal{W}_{\text{bend}}^{\text{local}}[\theta, \tilde{\theta}, l_e, l_1, l_2, r_1, r_2] = \frac{(\theta - \tilde{\theta})^2}{d_e(l_e, l_1, l_2, r_1, r_2)} l_e^2. \quad (8)$$

Note, that in the derivatives below we will again use auxiliary variables, which are different from before and will be defined afterwards.

#### 3.1 First derivatives

For the first derivatives, we obtain

$$\begin{aligned} \partial_{\theta} \mathcal{W}_{\text{bend}}^{\text{local}} &= \frac{2l_e^2(\theta - \tilde{\theta})}{d_e}, \\ \partial_{\tilde{\theta}} \mathcal{W}_{\text{bend}}^{\text{local}} &= -\frac{2l_e^2(\theta - \tilde{\theta})}{d_e}, \\ \partial_{l_e} \mathcal{W}_{\text{bend}}^{\text{local}} &= \frac{l_e(\theta - \tilde{\theta})^2}{6d_e^2} \left( -l_e^2 \left( \frac{Y_6}{4A_l} + \frac{Y_5}{4A_r} \right) + 12d_e \right), \\ \partial_{r_1} \mathcal{W}_{\text{bend}}^{\text{local}} &= -\frac{l_e^2 r_1 (\theta - \tilde{\theta})^2 Y_4}{24d_e^2 A_r}, \\ \partial_{r_2} \mathcal{W}_{\text{bend}}^{\text{local}} &= -\frac{l_e^2 r_2 (\theta - \tilde{\theta})^2 Y_2}{24d_e^2 A_r}, \\ \partial_{l_1} \mathcal{W}_{\text{bend}}^{\text{local}} &= -\frac{l_e^2 l_1 (\theta - \tilde{\theta})^2 Y_3}{24d_e^2 A_l}, \text{ and} \\ \partial_{l_2} \mathcal{W}_{\text{bend}}^{\text{local}} &= -\frac{l_e^2 l_2 (\theta - \tilde{\theta})^2 Y_1}{24d_e^2 A_l}. \end{aligned}$$

### 3.2 Second derivatives

For the second derivatives, we obtain

$$\begin{aligned}
\partial_\theta \partial_\theta \mathcal{W}_{\text{bend}}^{\text{local}} &= 2 \frac{l_e^2}{d_e}, \\
\partial_{\tilde{\theta}} \partial_\theta \mathcal{W}_{\text{bend}}^{\text{local}} &= -2 \frac{l_e^2}{d_e}, \\
\partial_{l_e} \partial_\theta \mathcal{W}_{\text{bend}}^{\text{local}} &= \frac{l_e(\theta - \tilde{\theta})}{3d_e^2} \left( -l_e^2 \left( \frac{Y_6}{4A_l} + \frac{Y_5}{4A_r} \right) + 12d_e \right), \\
\partial_{r_1} \partial_\theta \mathcal{W}_{\text{bend}}^{\text{local}} &= -\frac{l_e^2 r_1(\theta - \tilde{\theta})}{12 A_r d_e^2} Y_4, \\
\partial_{r_2} \partial_\theta \mathcal{W}_{\text{bend}}^{\text{local}} &= -\frac{l_e^2 r_2(\theta - \tilde{\theta})}{12 A_r d_e^2} Y_2, \\
\partial_{l_1} \partial_\theta \mathcal{W}_{\text{bend}}^{\text{local}} &= -\frac{l_e^2 l_1(\theta - \tilde{\theta})}{12 A_l d_e^2} Y_3, \\
\partial_{l_2} \partial_\theta \mathcal{W}_{\text{bend}}^{\text{local}} &= -\frac{l_e^2 l_2(\theta - \tilde{\theta})}{12 A_l d_e^2} Y_1, \\
\partial_{\tilde{\theta}} \partial_{\tilde{\theta}} \mathcal{W}_{\text{bend}}^{\text{local}} &= 2 \frac{l_e^2}{d_e}, \\
\partial_{l_e} \partial_{\tilde{\theta}} \mathcal{W}_{\text{bend}}^{\text{local}} &= -\frac{l_e(\theta - \tilde{\theta})}{3d_e^2} \left( -l_e^2 \left( \frac{Y_6}{4A_l} + \frac{Y_5}{4A_r} \right) + 12d_e \right), \\
\partial_{r_1} \partial_{\tilde{\theta}} \mathcal{W}_{\text{bend}}^{\text{local}} &= \frac{l_e^2 r_1(\theta - \tilde{\theta})}{12 A_r d_e^2} Y_4, \\
\partial_{r_2} \partial_{\tilde{\theta}} \mathcal{W}_{\text{bend}}^{\text{local}} &= \frac{l_e^2 r_2(\theta - \tilde{\theta})}{12 A_r d_e^2} Y_2, \\
\partial_{l_1} \partial_{\tilde{\theta}} \mathcal{W}_{\text{bend}}^{\text{local}} &= \frac{l_e^2 l_1(\theta - \tilde{\theta})}{12 A_l d_e^2} Y_3, \\
\partial_{l_2} \partial_{\tilde{\theta}} \mathcal{W}_{\text{bend}}^{\text{local}} &= \frac{l_e^2 l_2(\theta - \tilde{\theta})}{12 A_l d_e^2} Y_1, \\
\partial_{l_e} \partial_{l_e} \mathcal{W}_{\text{bend}}^{\text{local}} &= \frac{(\theta - \tilde{\theta})^2}{72d_e^3} \left[ -48l_e^2 d_e \left( \frac{Y_6}{4A_l} + \frac{Y_5}{4A_r} \right) \right. \\
&\quad - 12d_e l_e^2 \left( -\frac{2l_e^2 Y_6^2}{64A_l^3} + \frac{-3l_e^2 + X_2}{4A_l} - \frac{2l_e^2 Y_5^2}{64A_r^3} + \frac{-3l_e^2 + r_1^2 + r_2^2}{4A_r} \right) \\
&\quad + 4l_e^4 \left( \frac{Y_6}{4A_l} + \frac{Y_5}{4A_r} \right)^2 \\
&\quad \left. + (12d_e)^2 \right],
\end{aligned}$$

$$\begin{aligned}\partial_{r_1}\partial_{l_e}\mathcal{W}_{\text{bend}}^{\text{local}} = & -\frac{3l_er_1(\theta-\tilde{\theta})^2}{16A_r^3A_l(12d_e)^3}\left[-l_e^{10}\right. \\ & + l_e^8(3r_1^2-r_2^2) \\ & + l_e^6(Z_1-3r_1^4+3r_2^4+4r_2^2X_2+X_1^2) \\ & - l_e^4(r_1^2(Z_1-3r_2^4-4r_2^2X_2+3X_1^2)+r_2^2(-3\cdot Z_1+r_2^4+4r_2^2X_2+3X_1^2)-r_1^6+3r_1^4r_2^2) \\ & - l_e^2X_3(r_1^2(Z_1-3X_1^2)+r_2^2(X_1^2-3\cdot Z_1)) \\ & \left.+ X_3^3(Z_1-X_1^2)\right],\end{aligned}$$

$$\begin{aligned}\partial_{r_2}\partial_{l_e}\mathcal{W}_{\text{bend}}^{\text{local}} = & -\frac{3l_el_2(\theta-\tilde{\theta})^2}{16A_r^3A_l(12d_e)^3}\left[-l_e^{10}\right. \\ & + l_e^8(3r_2^2-r_1^2) \\ & + l_e^6(Z_1-3r_2^4+3r_1^4+4r_1^2X_2+X_1^2) \\ & + l_e^4(r_2^2(-Z_1+r_2^4-3X_1^2)+r_1^2(3\cdot Z_1-3r_2^4+4r_2^2X_2-3X_1^2)-r_1^6+3r_1^4r_2^2-4r_1^4X_2) \\ & - l_e^2X_3(r_2^2(3X_1^2-Z_1)+r_1^2(3\cdot Z_1-X_1^2)) \\ & \left.- X_3^3(Z_1-X_1^2)\right],\end{aligned}$$

$$\begin{aligned}\partial_{l_1}\partial_{l_e}\mathcal{W}_{\text{bend}}^{\text{local}} = & -\frac{3l_el_1(\theta-\tilde{\theta})^2}{16A_l^3A_r(12d_e)^3}\left[-l_e^{10}\right. \\ & + l_e^8(3l_1^2-l_2^2) \\ & + l_e^6(Z_1-3l_1^4+3l_2^4+4l_2^2X_4+X_3^2) \\ & - l_e^4(l_1^2(Z_1-3l_2^4-4l_2^2X_4+3X_3^2)+l_2^2(-3\cdot Z_1+l_2^4+4l_2^2X_4+3X_3^2)-l_1^6+3l_1^4l_2^2) \\ & - l_e^2X_1(l_1^2(Z_1-3X_3^2)+l_2^2(X_3^2-3\cdot Z_1)) \\ & \left.+ X_1^3(Z_1-X_3^2)\right],\end{aligned}$$

$$\begin{aligned}\partial_{l_2}\partial_{l_e}\mathcal{W}_{\text{bend}}^{\text{local}} = & -\frac{3l_el_2(\theta-\tilde{\theta})^2}{16A_l^3A_r(12d_e)^3}\left[-l_e^{10}\right. \\ & + l_e^8(3l_2^2-l_1^2) \\ & + l_e^6(Z_1-3l_2^4+3l_1^4+4l_1^2X_4+X_3^2) \\ & + l_e^4(l_2^2(-Z_1+l_2^4-3X_3^2)+l_1^2(3\cdot Z_1-3l_2^4+4l_2^2X_4-3X_3^2)-l_1^6+3l_1^4l_2^2-4l_1^4X_4) \\ & - l_e^2X_1(l_2^2(3X_3^2-Z_1)+l_1^2(3\cdot Z_1-X_3^2)) \\ & \left.- X_1^3(Z_1-X_3^2)\right],\end{aligned}$$

$$\begin{aligned}
\partial_{r_1} \partial_{r_1} \mathcal{W}_{\text{bend}}^{\text{local}} &= \frac{6l_e^2(\theta - \tilde{\theta})^2}{(12d_e)^3} \left( -\frac{12d_e(l_e^2 - 3r_1^2 + r_2^2)}{A_r} + \frac{r_1^2 Y_4^2}{A_r^2} + \frac{3d_e r_1^2 Y_4^2}{2A_r^3} \right), \\
\partial_{r_2} \partial_{r_1} \mathcal{W}_{\text{bend}}^{\text{local}} &= -\frac{3}{2} \frac{l_e^2 r_1 r_2 (\theta - \tilde{\theta})^2}{A_r^3 (12d_e)^3} (-12l_e^4 d_e - 4l_e^4 A_r + 12l_e^2 X_4 d_e + 4X_3^2 A_r), \\
\partial_{l_1} \partial_{r_1} \mathcal{W}_{\text{bend}}^{\text{local}} &= \frac{l_e^2 l_1 r_1 (\theta - \tilde{\theta})^2 Y_3 Y_4}{18Z_1 d_e^3}, \\
\partial_{l_2} \partial_{r_1} \mathcal{W}_{\text{bend}}^{\text{local}} &= \frac{l_e^2 l_2 r_1 (\theta - \tilde{\theta})^2 Y_1 Y_4}{18Z_1 d_e^3}, \\
\partial_{r_2} \partial_{r_2} \mathcal{W}_{\text{bend}}^{\text{local}} &= \frac{6l_e^2(\theta - \tilde{\theta})^2}{(12d_e)^3} \left( -\frac{12d_e(l_e^2 + r_1^2 - 3r_2^2)}{A_r} + \frac{r_2^2 Y_2^2}{A_r^2} + \frac{3d_e r_2^2 Y_2^2}{2A_r^3} \right), \\
\partial_{l_1} \partial_{r_2} \mathcal{W}_{\text{bend}}^{\text{local}} &= \frac{l_e^2 l_1 r_2 (\theta - \tilde{\theta})^2 Y_3 Y_2}{18Z_1 d_e^3}, \\
\partial_{l_2} \partial_{r_2} \mathcal{W}_{\text{bend}}^{\text{local}} &= \frac{l_e^2 l_2 r_2 (\theta - \tilde{\theta})^2 Y_1 Y_2}{18Z_1 d_e^3}, \\
\partial_{l_1} \partial_{l_1} \mathcal{W}_{\text{bend}}^{\text{local}} &= \frac{6l_e^2(\theta - \tilde{\theta})^2}{(12d_e)^3} \left( -\frac{12d_e(l_e^2 - 3l_1^2 + l_2^2)}{A_l} + \frac{l_1^2 Y_3^2}{A_l^2} + \frac{3d_e l_1^2 Y_3^2}{2A_l^3} \right), \\
\partial_{l_2} \partial_{l_1} \mathcal{W}_{\text{bend}}^{\text{local}} &= -\frac{3}{2} \frac{l_e^2 l_1 l_2 (\theta - \tilde{\theta})^2}{A_l^3 (12d_e)^3} (-12l_e^4 d_e - 4l_e^4 A_l + 12l_e^2 X_2 d_e + 4X_1^2 A_l), \text{ and} \\
\partial_{l_2} \partial_{l_2} \mathcal{W}_{\text{bend}}^{\text{local}} &= \frac{6l_e^2(\theta - \tilde{\theta})^2}{(12d_e)^3} \left( -\frac{12d_e(l_e^2 + l_1^2 - 3l_2^2)}{A_l} + \frac{l_2^2 Y_1^2}{A_l^2} + \frac{3d_e l_2^2 Y_1^2}{2A_l^3} \right).
\end{aligned}$$

The remaining derivatives follow by symmetry.

### 3.3 Auxiliary variables

$$\begin{aligned}
X_1 &:= l_1^2 - l_2^2 & Y_1 &:= l_e^2 + X_1 & Z_1 &:= 4A_l 4A_r \\
X_2 &:= l_1^2 + l_2^2 & Y_2 &:= l_e^2 + X_3 \\
X_3 &:= r_1^2 - r_2^2 & Y_3 &:= l_e^2 - X_1 \\
X_4 &:= r_1^2 + r_2^2 & Y_4 &:= l_e^2 - X_3 \\
&& Y_5 &:= -l_e^2 + X_4 \\
&& Y_6 &:= -l_e^2 + X_2
\end{aligned}$$
